# Supplementary material for: Squeezed thermal reservoirs as a resource for a nano-mechanical engine beyond the Carnot limit
Source: arXiv:1703.10024 ancillary file (2017-04-25)
Supplement: Supplementary file 1 [file supplemental.pdf]

# Supplemental Material

## Squeezed thermal reservoirs as a resource for a nano-mechanical engine beyond the Carnot limit

Jan Klaers[1§], Stefan Faelt[1], Atac Imamoglu[1], and Emre Togan[1]

[1]*Institute of Quantum Electronics, ETH Zürich, CH-8093 Zürich, Switzerland*

[§]*Corresponding author. Email: jklaers@phys.ethz.ch*

## 1 Theoretical background

We summarize statistical and thermodynamical properties of a single harmonic oscillator coupled to a squeezed thermal bath and derive the efficiency of an Otto cycle operating between two squeezed thermal reservoirs.

### Basic properties

We consider a harmonic oscillator with angular frequency $\omega$ coupled to a squeezed thermal bath [23, 24, 25, 33, 34, 35, 36]. In a steady-state, the oscillator can be expected to follow temperature $T$ and squeezing $r$ of the bath. This scenario is best described in a position-momentum-frame $(x_0, p_0)$ that rotates with frequency $\omega$ with respect to the laboratory frame. In this frame, the probability of finding the oscillator at position $x_0$ follows a Gaussian distribution with variance proportional to the temperature $T_1$, whereas the momentum distribution is Gaussian with variance proportional to $T_2$:

$$\rho(x_0) = \sqrt{\frac{\hbar\omega}{2\pi k_\mathrm{B} T_1}} \exp\left(-\frac{\hbar\omega x_0^2}{2k_\mathrm{B}T_1}\right) \qquad \text{(S1)}$$

$$\rho(p_0) = \sqrt{\frac{\hbar\omega}{2\pi k_\mathrm{B} T_2}} \exp\left(-\frac{\hbar\omega p_0^2}{2k_\mathrm{B}T_2}\right) \qquad \text{(S2)}$$

We use the convention that the position quadrature $x_0$ corresponds to the anti-squeezed quadrature, whereas the momentum quadrature corresponds to the squeezed quadrature. The parameters $T_{1,2}$ are connected to temperature $T$ and squeezing parameter $r$ of the system via

$$T_{1,2} = T\,\exp(\pm 2r)\;, \tag{S3}$$

which for vanishing squeezing describes a purely thermal state with identical fluctuations in each quadrature, that is $T_1 = T_2 = T$.

### Caloric equation of state

The internal energy of the harmonic oscillator follows from eqs. (S1)-(S3) as

$$\begin{aligned} U &= \int_{-\infty}^{+\infty}\int_{-\infty}^{+\infty} \rho(x_0)\rho(p_0)\,(\hbar\omega/2)(x_0^2+p_0^2)\,dx_0 dp_0 \\ &= \frac{k_\mathrm{B}}{2}(T_1+T_2) \qquad \text{(S4)} \\ &= k_\mathrm{B}T(1+2\sinh^2 r)\;. \qquad \text{(S5)} \end{aligned}$$

### Energy distribution function

Based on eq. (S1) and (S2), the probability of finding the position or momentum quadrature in a state with energy $e$ is given by $p_i(e) \propto \exp(-e/k_\mathrm{B}T_i)/\sqrt{e}$ for $i = 1,2$, where the factor $1/\sqrt{e}$ represents the density of states. Correspondingly, the probability of finding the squeezed harmonic oscillator in a state with total energy $E$ (sum over both quadratures) is given by

$$\begin{aligned} \rho(E) &= z^{-1}\int_0^E \rho_1(e)\,\rho_2(E-e)\,de \\ &= \frac{1}{k_\mathrm{B}T}\,I_0\left(\frac{E\,\sinh 2r}{k_\mathrm{B}T}\right)\,\exp\left(-\frac{E\,\cosh 2r}{k_\mathrm{B}T}\right) \qquad \text{(S6)} \end{aligned}$$

where $I_0(x)$ is the modified Bessel function of order zero and the normalization constant $z$ has been chosen such that $\int_0^\infty \rho(E)\,dE = 1$.

### Entropy (First method)

For a thermodynamic description of the harmonic oscillator in a squeezed thermal state, we introduce three state variables: two entropy variables $S_{1,2}$, one for each quadrature, and the volume parameter $V = 1/\omega$. With this, the internal energy may be written as $U = U(S_1, S_2, V)$. Analogous to standard thermodynamic expressions, we define

$$T_1 = \left(\frac{\partial U}{\partial S_1}\right)_{S_2,V} \tag{S7}$$

$$T_2 = \left(\frac{\partial U}{\partial S_2}\right)_{S_1,V} \tag{S8}$$

$$p = -\left(\frac{\partial U}{\partial V}\right)_{S_1,S_2} . \tag{S9}$$

Starting from the caloric equation of state, one can derive the following partial differential equation

$$\begin{aligned} U(S_1,S_2,V) &\overset{\text{eq. }S4}{=} \frac{k_\mathrm{B}}{2}(T_1+T_2) \\ &\overset{\text{eq. }S7,S8}{=} \frac{k_\mathrm{B}}{2}\left[\left(\frac{\partial U}{\partial S_1}\right)_{S_2,V} + \left(\frac{\partial U}{\partial S_2}\right)_{S_1,V}\right] \end{aligned}$$

The internal energy may be written as sum of two energy contributions originating from squeezed and anti-squeezed quadrature

$$U(S_1,S_2,V) = U_1(S_1,V) + U_2(S_2,V) . \tag{S10}$$

Using this ansatz, we find

$$U_1(S_1,V) + U_2(S_2,V) = \frac{k_\mathrm{B}}{2}\left[\left(\frac{\partial U_1}{\partial S_1}\right)_V + \left(\frac{\partial U_2}{\partial S_2}\right)_V\right] . \tag{S11}$$

Considering $S_1$ and $S_2$ as independent variables, this partial differential equation is solved by

$$\begin{aligned} U_1(S_1,V) &= \exp(2S_1/k_\mathrm{B})\, f_1(V) + f_2(V) \\ U_2(S_2,V) &= \exp(2S_2/k_\mathrm{B})\, f_3(V) - f_2(V) \end{aligned}$$

with three a priori unknown functions $f_i(V)$ for $i = 1,2,3$. Changing the sign of the squeezing parameter $r \to -r$, should reverse the roles of $U_1$ and $U_2$. Thus, one has to demand $f_1 = f_3$ and $f_2 = 0$. The only remaining unknown function $f_1$ can finally be determined by correspondence with the known entropy of an unsqueezed thermal state $S = k_\mathrm{B}(\ln(U/\hbar\omega)+1)$, which arises for $S_1 = S_2 = S/2$. This gives $f_1 = e^{-1}\,\hbar\omega/2 = e^{-1}\,\hbar/2V$ and thus

$$U_i = \hbar/2V\ \exp(2S_i/k_\mathrm{B} - 1) \tag{S12}$$

for $i = 1,2$. Solving for the entropy, we arrive at the expression

$$S_i = \frac{k_\mathrm{B}}{2}\left(\ln\left(2U_iV/\hbar\right)+1\right) = \frac{k_\mathrm{B}}{2}\left(\ln\left(2U_i/\hbar\omega\right)+1\right) = \frac{k_\mathrm{B}}{2}\left(\ln\left(k_\mathrm{B}T_i/\hbar\omega\right)+1\right) . \tag{S13}$$

For the total entropy $S = S_1 + S_2$, it follows

$$S = k_{\mathrm{B}} \left( \ln \left( 2\sqrt{U_1 U_2}/\hbar\omega \right) + 1 \right) = k_{\mathrm{B}} \left( \ln \left( k_{\mathrm{B}} T/\hbar\omega \right) + 1 \right) . \tag{S14}$$

Note that the total entropy is unaffected by the squeezing parameter. An isothermal squeezing operation applied to a purely thermal state does not increase its entropy.

## Entropy (Second method)

We give a second derivation of eq. (S13). For this, we interpret the entropies $S_{1,2}$ as Shannon entropies, for example

$$\begin{aligned} S_1 &= -k_{\mathrm{B}} \int_{-\infty}^{+\infty} \rho(x_0) \ln(\rho(x_0))\, dx_0 \\ &\overset{\mathrm{eq.}\, S1}{=} \frac{k_{\mathrm{B}}}{2} \left( \ln \left( k_{\mathrm{B}} T_1/\hbar\omega \right) + 1 + \ln(2\pi) \right) \end{aligned} \tag{S15}$$

(and analogous for $S_2$). Besides an additional offset of $\ln(2\pi)\, k_{\mathrm{B}}/2$, this result agrees with eq. (S13). For the purpose of this work, for which a calibration to absolute entropy values is not required, both expressions can be regarded as equivalent.

## Free Energy

By means of two Legendre transforms one can obtain the free energy of a squeezed thermal state

$$\begin{aligned} F &= U - T_1 S_1 - T_2 S_2 \\ &\overset{\mathrm{eq.}\, S13, S3}{=} -k_{\mathrm{B}} T \left( 1 + 2\sinh^2 r \right) \ln(k_{\mathrm{B}} T V/\hbar) - 2 k_{\mathrm{B}} T\, r \sinh 2r \, . \end{aligned} \tag{S16}$$

The free energy of a squeezed thermal state explicitly depends on the squeezing parameter recovering the case of an unsqueezed thermal oscillator $F = -k_{\mathrm{B}} T \, \ln(k_{\mathrm{B}} T/\hbar\omega)$ for $r = 0$. While an isothermal squeezing operation applied to a purely thermal state does not alter its entropy, isothermal squeezing causes a change in free energy indicating that squeezed thermal states allow for larger work extraction than purely thermal states at the same temperature.

## "First law"

An equation analogous to the state functional formulation of the first law of thermodynamics holds:

$$\begin{aligned} dU &\overset{\mathrm{eq.}\, S10}{=} dU_1 + dU_2 \\ &\overset{\mathrm{eq.}\, S7, S8}{=} T_1 dS_1 - p_1 dV + T_2 dS_2 - p_2 dV \\ &= T_1 dS_1 + T_2 dS_2 - (p_1 + p_2)\, dV \\ &= T_1 dS_1 + T_2 dS_2 - p dV \, . \end{aligned} \tag{S17}$$

In the last three steps, we additionally have employed $p = p_1 + p_2$ with $p_i = -\left(\partial U_i / \partial V\right)_{S_i}$ for $i = 1, 2$. Thus, the term $-p\,dV$ represents the work associated to a change in volume, while the terms $T_i\,dS_i$ with $i = 1, 2$ describe heat exchange with the bath.

## Thermal equation of state (First method)

Following eq. (S12), the internal energy may be written as

$$U(S_1, S_2, V) = \frac{\hbar}{2V}\left(\exp\left(2S_1/k_\mathrm{B} - 1\right) + \exp\left(2S_2/k_\mathrm{B} - 1\right)\right) . \tag{S18}$$

For the pressure, it follows

$$\begin{aligned} p &= -\left(\frac{\partial U}{\partial V}\right)_{S_1, S_2} \\ &= \frac{\hbar}{2}\frac{1}{V^2}\left(\exp\left(2S_1/k_\mathrm{B} - 1\right) + \exp\left(2S_2/k_\mathrm{B} - 1\right)\right) \\ &\overset{\text{eq.}\,S13}{=} \frac{k_\mathrm{B}}{2}\frac{(T_1 + T_2)}{V} . \end{aligned}$$

This gives the thermal equation of state $p\,V = U$, or

$$p\,V = k_\mathrm{B} T\left(1 + 2\sinh^2 r\right) . \tag{S19}$$

## Thermal equation of state (Second method)

During an ideal adiabatic expansion or compression of the harmonic oscillator there is no contact to a thermal reservoir. One would expect the number of phonons to remain constant during such as process (particle number conservation). The latter suggests that the phonon number $\bar{n}$ of a squeezed thermal state (written as a function of the state variables $S_1$, $S_2$, $V = \omega^{-1}$) should solely depend on the entropies $S_{1,2}$, which remain constant during an adiabatic step, and not on the volume $V$. This may be expressed as

$$\bar{n}(S_1, S_2, V) = \bar{n}(S_1, S_2) .$$

The internal energy is then given by

$$U(S_1, S_2, V) = \hbar\omega\,\bar{n}(S_1, S_2) . \tag{S20}$$

With the definition of the pressure eq. (S9), the thermal equation of state $p = U/V$ immediately follows.

## Otto cycle with squeezed thermal baths [17, 37]

We consider an Otto cycle at maximum power operating between a hot squeezed thermal reservoir with temperature and squeezing parameter $(T_\mathrm{h}, r_\mathrm{h})$ and a cold squeezed thermal reservoir with parameters $(T_\mathrm{c}, r_\mathrm{c})$, see Fig. S1a .

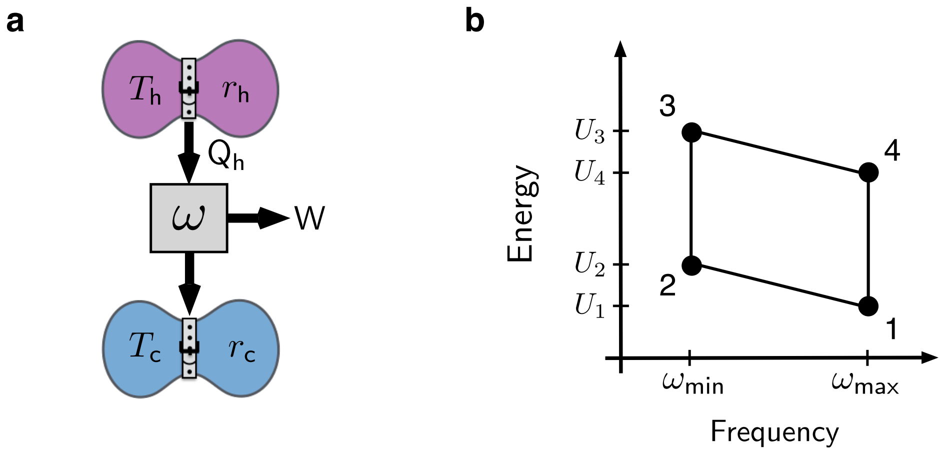


Figure S1: **a**, Otto cycle performed with a single harmonic oscillator with (tunable) frequency $\omega$ coupled to two squeezed reservoirs. **b**, Energy-frequency diagram of the Otto cycle.

The working medium consists of a single harmonic oscillator with (tunable) frequency $\omega$. The cycle includes four strokes

| Path | Type | Heat | Work |
|---|---|---|---|
| $1 \to 2$ | adiabatic compression | $Q_{12} = 0$ | $W_{12} = U_2 - U_1$ |
| $2 \to 3$ | isochoric heat addition | $Q_{23} = U_3 - U_2$ | $W_{23} = 0$ |
| $3 \to 4$ | adiabatic expansion | $Q_{34} = 0$ | $W_{34} = U_4 - U_3$ |
| $4 \to 1$ | isochoric heat rejection | $Q_{41} = U_4 - U_1$ | $W_{41} = 0$ |

where the energies $U_i$ (Fig. S1b) follow from the caloric equation of state eq. (S5) with

| Point | Temperature | Squeezing |
|---|---|---|
| 1 | $T = T_\mathrm{c}$ | $r = r_\mathrm{c}$ |
| 2 | $T = T_\mathrm{c}\,(\omega_\mathrm{min}/\omega_\mathrm{max})$ | $r = r_\mathrm{c}$ |
| 3 | $T = T_\mathrm{h}$ | $r = r_\mathrm{h}$ |
| 4 | $T = T_\mathrm{h}\,(\omega_\mathrm{max}/\omega_\mathrm{min})$ | $r = r_\mathrm{h}$ |

The total amount of work per cycle is given by $W = -\sum W_{ij} = -U_2 + U_1 - U_4 + U_3$, or

$$W = \left(1 - \frac{\omega_{\rm max}}{\omega_{\rm min}}\right) k_{\rm B} T_{\rm h} \cosh^2 r_{\rm h} + \left(1 - \frac{\omega_{\rm min}}{\omega_{\rm max}}\right) k_{\rm B} T_{\rm c} \cosh^2 r_{\rm c} \, .$$

We now select the frequency ratio $\omega_{\rm max}/\omega_{\rm min}$ that maximizes $W$ (maximum power condition). This is given for

$$\left(\frac{\omega_{\rm max}}{\omega_{\rm min}}\right)_{\rm max.\ power} = \frac{\cosh r_{\rm h}}{\cosh r_{\rm c}} \sqrt{\frac{T_{\rm h}}{T_{\rm c}}} \, . \tag{S21}$$

Finally, the efficiency $\eta = W/Q_{23}$ of the Otto cycle follows as

$$\eta = 1 - \sqrt{\frac{T_{\rm c}}{T_{\rm h}}} \frac{\cosh r_{\rm c}}{\cosh r_{\rm h}} \, . \tag{S22}$$

In the experimental realization, we haven chosen $r_{\rm c} = 0$ and $r_{\rm h} = r$, which results in $\eta = 1 - \sqrt{T_{\rm c}/T_{\rm h}} \,/\cosh(r)$. For vanishing squeezing the Curzon-Ahlborn limit is recovered, while for $r \to \infty$ the efficiency goes to unity.

# 2 Experimental methods & additional data analysis

## Nano-beam oscillator

The experimental setup is a physical implementation of a (single) frequency-tunable harmonic oscillator coupled to a squeezed thermal bath. The mechanical oscillator is realized by the fundamental flexural mode (out-of-plane bending) of a doubly-clamped gallium arsenide (GaAs) nano-beam structure with eigenfrequency $\nu = \omega/2\pi = 1.97\,$MHz and quality factor of order $Q \simeq 10^3$ at room temperature and under vacuum conditions ($p \simeq 10^{-4}\,$mbar), see Fig. S2a. The beam has a length of $18.8\,\mu$m, width of $2\,\mu$m, thickness of 270 nm, and is fabricated using conventional nano-structuring techniques such as electron beam lithography and selective etching. The structure contains two doped layers which can be electrically contacted to apply an electric field across the beam perpendicular to the sample plane. Due to the piezo-electricity of gallium arsenide, an applied AC electrical field generates a periodic mechanical force that can lead to actuation of mechanical vibrations.

Furthermore, by applying a DC bias voltage between the doped layers, the frequency of the mechanical oscillation becomes tunable, as is demonstrated in Fig. S2b. In our sample geometry, the inverse piezo-electric effect generates a compressive load on the nano-beam which alters its resonance frequency (softening of the effective spring constant). This frequency change does not occur instantaneously. Experimentally, we find that the switching of the nano-beam frequency follows an exponential decay with time constant 3.5µs (in response to a step-like change of the applied voltage). This is roughly a factor 6 slower than the oscillation period of the oscillator. For this reason, AC electrical fields (noise) at the resonance frequency mostly acts as additive force and not as parametric noise.

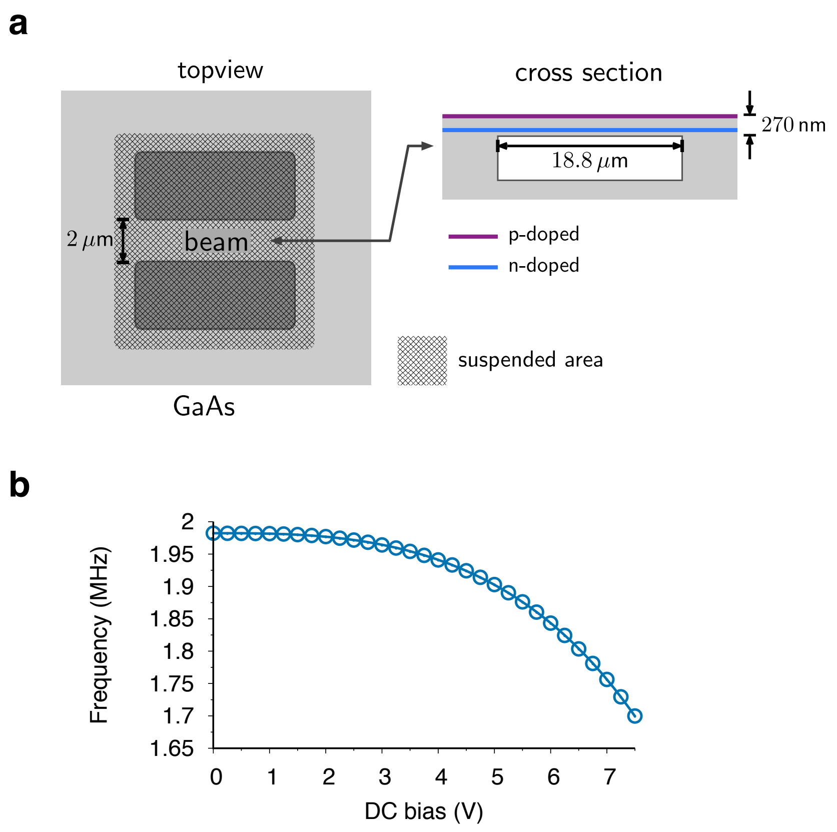


Figure S2: **a**, Doubly-clamped GaAs nano-beam structure as mechanical oscillator. **b**, Mechanical eigenfrequency of the fundamental flexural mode of the nano-beam as a function of the applied DC bias voltage (circles). The solid line shows a polynomial interpolation.

## Squeezed thermal reservoir

A squeezed thermal environment for the nano-beam oscillator is mimicked by engineered electronic noise, see Fig. S3, that couples to the nano-beam motion via the piezo-electricity of GaAs, and is synthesized from two independent white noise signals $\xi_{1,2}(t)$ that are mixed with sine and cosine component of a phase reference at the mechanical eigenfrequency $\nu = \omega/2\pi$. This leads to a stochastic force

$$f(t) = a_0 \left[ \mathrm{e}^{+\tilde{r}} \xi_1(t) \cos(\omega t + \phi) + \mathrm{e}^{-\tilde{r}} \xi_2(t) \sin(\omega t + \phi) \right] \tag{S23}$$

being applied to the oscillator, as is described by the Langevin equation

$$m \frac{d^2 x(t)}{dt^2} = -\frac{\partial U(x(t))}{\partial x} - \gamma \frac{dx(t)}{dt} + f(t) \tag{S24}$$

where $m$ denotes the (effective) mass of the oscillator, $U(x) = m\omega^2 x^2/2$ describes the harmonic confining potential, and $\gamma$ denotes the damping (e.g. losses to the environment through the clamps). The squeezed heat bath is characterized by an overall amplitude $a_0$, a squeezing control parameter $\tilde{r}$ and a phase factor $\phi$. In the experiments, the parameters $a_0$ and $\tilde{r}$ are used to adjust temperature and squeezing of the nano-beam motion according to the intended cyclic process. To remove non-resonant contributions, we restrict the bandwidth of the noise to 10 kHz around the mechanical resonance.

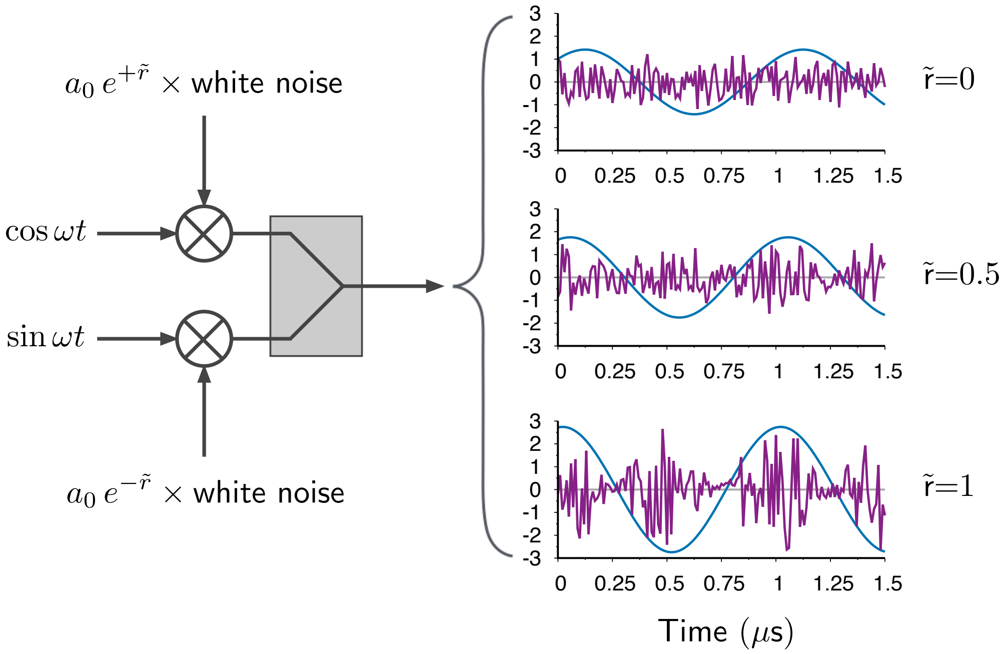


Figure S3: Experimental scheme to provide a squeezed thermal bath (left). Examples of squeezed noise $f(t)$ at a frequency of $\omega = 2\pi \cdot 2\,\mathrm{MHz}$ for three different squeezing factors (purple lines). A phase reference for these baths may be derived from $f_{\mathrm{ref}}(t) = a_0 \left[\mathrm{e}^{+\tilde{r}} \cos(\omega t + \phi) + \mathrm{e}^{-\tilde{r}} \sin(\omega t + \phi)\right]$ (blue lines).

## Detection of motional state

The motional state of the nano-beam is measured using a Mach-Zehnder interferometer (balanced homodyne detection). We use an external cavity single-frequency laser operating at a wavelength of $\lambda = 1550\,\mathrm{nm}$ with a power of $p_{\mathrm{Laser}} \simeq 100\,\mu\mathrm{W}$ as interferometer laser. The out-of-plane displacement of the beam, which in our experiments is typically below (or of order) of 1 nm, alters the length of one interferometer arm leading to small intensity modulations at the frequency $\nu$ of the mechanical oscillator in the two interferometer outputs. The amplified difference signal is down-converted by mixing with a local oscillator at a frequency of $\nu_{\mathrm{loc}} = \nu - 20\,\mathrm{kHz}$ and digitized by a software defined

radio receiver with a sample rate of 25 MS/s. The digitized data is purified by means of a spectral filter which suppresses spectral signals outside the bandpass region [$\nu$-10 kHz, $\nu$+10 kHz]. The signal so obtained describes the position $x(t)$ of the nano-beam up to a proportionality factor, and can be used to determine all other quantities of interest such as velocities, energies, temperatures, etc.. Absolute values are obtained by normalizing the measurement signals to known values obtained for a system without additional drive ($a_0 = 0$) [38]. For example, an absolute energy scale is obtained by normalizing the measurement of the mean energy of the oscillator for an undriven system to the known value of $k_B T \simeq 25$ meV at room temperature. The temperatures for anti-squeezed and squeezed quadrature $T_{1,2}$ are derived from the Gaussian widths of position and momentum distribution $\rho(x_0)$, $\rho(p_0)$. From this, we further infer the system temperature $T = \sqrt{T_1 T_2}$ and squeezing parameter $r = \ln(T_1/T_2)/4$.

## Error bars and data averaging

In the experiments, the engine quasi-statically runs through the engine protocol (cycle times amount to several seconds). At each point of the cycle that is represented by a data point (e.g. in Fig. 2a,b,c), the state of the system is recorded for 0.5 seconds during one iteration of the cycle. In total, after completing several cycles, each data point corresponds to an average of 20 to 40 seconds of integration. Except for the oscillator frequency, which is essentially known to 'arbitrary' precision, and Fig. 2c (for the clarity of presentation), the statistical uncertainties in the data points in Fig. 2 and Fig. 3 are indicated by error bars, which in most cases are smaller than the symbol size. All error bars represent the standard error of the mean (s.e.m.) except for the error bars in Fig. 2d, which are based on error estimates derived from a curve fitting procedure. For the latter, we first determine polynomial fit functions (up to second order) to the pressure-volume and temperature-entropy data points (Figures 2b and 2c) belonging to one stroke of the engine cycle. The uncertainties of the fit parameters are then used to obtain error estimates of the work output $W$, heat consumptions $Q_{1,2}$ and efficiency $\eta = W/(Q_1 - Q_2)$.

## Otto cycle with squeezed heat

In Fig. 2 of the main text we present experimental results that characterize an Otto cycle between a hot squeezed bath at temperature $T_h = 10,000$ K with squeezing parameter $r$ and a cold purely thermal bath at temperature $T_c = 9,500$ K. The cycle process is performed under maximum power conditions meaning that minimum and maximum frequency (volume) of the nano-beam oscillator are connected by $\nu_{max}/\nu_{min} = \cosh r \sqrt{T_h/T_c}$, see eq. (S21). For the minimum frequency we choose $\nu_{min} = 1.77$ MHz in all seven data sets. The cycle includes two adiabatic steps and two isochores. The adiabatic compression and expansion are implemented as isentropic steps, meaning that, instead of decoupling the system from the heat bath, we simultaneously vary frequency and temperature keeping the entropy of the state fixed [9]. More specifically, in steps (A) and (C) of Fig. 2 we vary temperature and frequency keeping the ratio $T_i/\omega$ constant (for $i = 1, 2$), which conserves the entropies in each quadrature and the total entropy, see eq. (S13) and (S14) and Fig. S4.

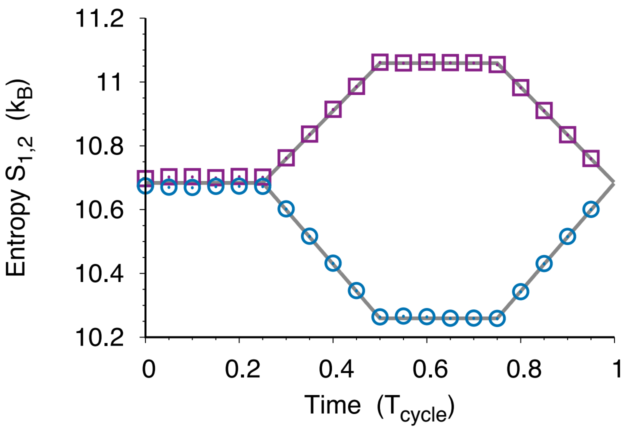


Figure S4: Entropy of squeezed (circles) and anti-squeezed quadrature (boxes) as a function of time during the Otto cycle presented in Fig. 2 of the main text. Note that within the experimental uncertainties [statistical errors (s.e.m.) are smaller than the symbol size], the entropy in both quadratures stays fixed during the isentropic steps (first and third quarter of the cycle). The solid line represents the theoretically expected behavior. Experimental parameters are as described in Fig. 2 of the main text.

### Extraction of work from a single reservoir

In Fig. 3 of the main text, we present experimental results characterizing the extraction work from a single squeezed reservoir. For these experiments, we introduce a phase-selective thermal coupling between mechanical oscillator and squeezed heat bath. The relative phase between coupling and squeezed bath effectively determines the temperature/energy of the oscillator. The $T-S$ diagram of this cycle is presented in Fig. S5. The shaded area corresponds to the heat exchange of the anti-squeezed quadrature (boxes) of the mechanical oscillator with the reservoir per cycle. Using polynomial fits to the data points (solid lines), we interpolate the boundaries of this area and determine a net heat consumption of $Q \simeq (33 \pm 11)$ meV. The conservation of energy (first law of thermodynamics) requires that this energy balances the extracted work. Indeed, the obtained value is consistent with the corresponding work output of $W = (37 \pm 2)$ meV per cycle as inferred from the $P-V$ diagram of Fig. 3c. The anti-squeezed quadrature (circles) does not significantly contribute to the heat exchange.

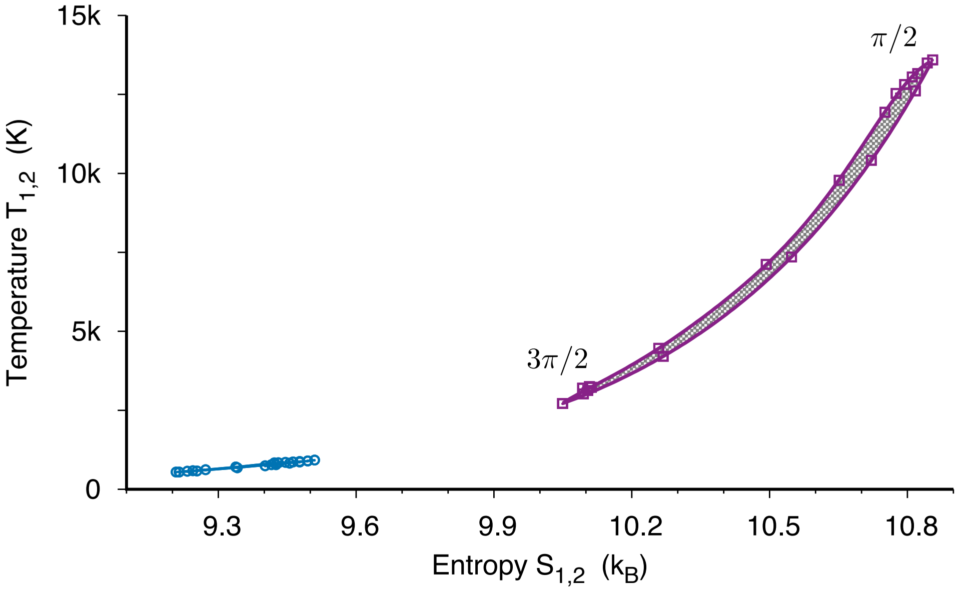


Figure S5: $T - S$ diagram of the engine cycle presented in Fig. 3 of the main text. The shaded area corresponds to the heat exchange of the anti-squeezed quadrature (boxes) of the mechanical oscillator with the reservoir per cycle. Using polynomial fits to the data points (lines), we interpolate the boundaries of this area and derive a net heat consumption of $Q \simeq (33 \pm 11)$ meV. The anti-squeezed quadrature (circles) does not significantly contribute to the heat exchange.

# References

[33] J. Oz-Vogt, A. Mann, and M. Revzen, *Thermal coherent states and thermal squeezed states*, J. Mod. Opt. **38**, 2339 (1991).

[34] B. G. Wang and J. X. Zhu, *Wigner functions for coherent and squeezed states with thermal noise*, J. Mod. Opt. **40**, 1917 (1993).

[35] P. Marian and T. A. Marian, *Squeezed states with thermal noise. I. Photon-number statistics*, Phys. Rev. A **47**, 4474 (1993).

[36] P. Marian and T. A. Marian, *Squeezed states with thermal noise. II. Damping and photon counting*, Phys. Rev. A **47**, 4487 (1993).

[37] O. Abah, *Quantum machines at the nanoscale* (Doctoral dissertation, Friedrich-Alexander-Universität Erlangen-Nürnberg (FAU), 2015).

[38] B. D. Hauer, C. Doolin, K. S. D. Beach, and J. P. Davis, *A general procedure for thermomechanical calibration of nano/micro-mechanical resonators*, Ann. Phys. **339**, 181 (2013).
